# Supplementary material for: Fano Resonances in Mid-Infrared Spectra of Single-Walled Carbon Nanotubes
Source: arXiv:1203.3224 source file (2012-03-14)
Supplement: Supplementary file 1 [file irfanocnt_suppinfo_PRL_v5.pdf]

# Supplementary Material for "Fano Resonances in Mid-Infrared Spectra of Single-Walled Carbon Nanotubes"

François Lapointe, Étienne Gaufrès, Isabelle Tremblay, Nathalie Y-Wa Tang, and Richard Martel*
*Département de chimie, Université de Montréal, C. P. 6128,*
*Succursale Centre-Ville, Montréal, Québec H2C 3J7, Canada and*
*Regroupement Québécois sur les Matériaux de Pointe (RQMP)*

Patrick Desjardins
*Département de génie physique, École Polytechnique de Montréal, Montréal,*
*C. P. 6079, Succursale Centre-ville, Montréal, Québec H3C 3A7, Canada and*
*Regroupement Québécois sur les Matériaux de Pointe (RQMP)*

This work revisits the physics giving rise to the carbon nanotubes phonon bands in the mid-infrared. Our measurements of doped and undoped samples of single-walled carbon nanotubes in Fourier transform infrared spectroscopy show that the phonon bands exhibit an asymmetric lineshape and that their effective cross-section is enhanced upon doping. We relate these observations to electron-phonon coupling or, more specifically, to a Fano resonance phenomenon. We note that only dopant-induced intra-band transitions couple to the phonon modes and that defects induced in the sidewall increase the resonance probabilities.

## METHODOLOGY

### Purification and suspension

Laser ablation single-walled carbon nanotubes (SWNTs) (Benoit Simard, NRC Steacie Institute, Ottawa) were purified using a process described elsewhere [1]. Briefly, 100 mg of SWNTs were refluxed in concentrated nitric acid (70%, Certified ACS Plus, Fisher Scientific) for four hours, and filtrated over a PTFE membrane (pore size 1.2 $\mu$m, Sartorius Stadim Biotech). The SWNTs were then dispersed in deionized water (Millipore Milli-Q, 18.2 M$\Omega$), refluxed overnight, and filtrated again over a PTFE membrane.

The resulting SWNTs were dispersed in a 1% w/V sodium cholate solution (from ox or sheep bile, $\geq$99%, Sigma-Aldrich) in deionized water. The dispersion was submitted to ultrasonification for 30 min. in a bath (VWR Model 75D) and 30 min. using a high power microtip (Branson Sonifier 450, 400 watt, duty cycle 50%, output 3). Afterward, we used ultracentrifugation (20,800 rpm, one hour, 100,000 g, Beckman L8-70, rotor SW 41 Ti) to remove bundles and denser material from the dispersion. The supernatant was kept and the suspension was found to be stable over months.

### Films

Films of SWNTs were made using a procedure developed by Wu *et al.* [2] Three milliliters of the suspension were filtrated over mixed cellulose ester / cellulose nitrate filters (0.22 $\mu$m, Millipore GSTF-047-00). The films can be transferred to a convenient substrate by dissolving the filter in acetone (Certified ACS, Fisher Scientific) for 30 min.

### Annealing

Further cleaning and de-doping of the SWNT films was performed by annealing in a vacuum quartz tube furnace at 1100 K. The quality of the vacuum was maintained between $2\times10^{-5}$ and $2\times10^{-6}$ mbar using a turbomolecular pump. The spectra of the intrinsic state of the SWNTs films were taken right after annealing because it is known that the oxygen / water redox couple is a $p$ type dopant for SWNTs [3].

### Doping

Three different oxidizers were chosen for doping SWNT. 2,3-Dichloro-5,6-dicyano-1,4-benzoquinone (DDQ, 98%, Sigma-Aldrich) and iron(III) chloride hexahydrate ($FeCl_3\cdot 6H_2O$, $\geq$98%, Sigma-Aldrich) solutions were made at a concentration of 25 mM in acetonitrile (reagent grade, American Chemicals Ltd). Thionyl chloride ($SOCl_2$, 99+%, American Chemicals Ltd) was used in pure form. The SWNTs films were left in the dopant for two days, rinsed in acetonitrile, dried with a $N_2$ stream, and the spectra were performed shortly after their removal from solution.

### Bromophenyl Functionalization

A solution at a concentration of 0.79 mM of 4-bromobenzenediazonium tetrafluoroborate (96%, Sigma-Aldrich) was prepared with degassed deionized water (Millipore Milli-Q, 18.2 M$\Omega$) and the pH was adjusted to $\sim$10 with NaOH [4]. The SWNT film was dipped into the aqueous salt solution for 10 minutes, rinsed with water, then with 2-propanol (Certified ACS Plus, Fisher

Scientific) and finally dried using a $N_2$ stream. The film was subsequently doped by immersion in a 1 mM DDQ solution in acetonitrile for 30 min.

## NIR-vis Spectroscopy

Spectra in the NIR-vis domain were performed using a Brüker Vertex 80v Fourier transform spectrometer. Two different spectral ranges were stitched together to cover the whole domain. From 0.5 to 1.4 eV, a tungsten source, $CaF_2$ beamsplitter and thermoelectric cooled InGaAs detector (Electro-optical Systems Inc.) were used. The resolution was set to 16 $cm^{-1}$, the HeNe modulation frequency to 10 kHz, and 1024 scans were averaged.

A room temperature silicon diode (Br"uker) was used as a detector from 1.2 to 3.0 eV, along with a NIR short pass filter. In this case, the resolution was 32 $cm^{-1}$, the HeNe modulation frequency was 10 kHz, and 512 scans were averaged.

We used quartz slides (ChemGlass) as a substrate for the NIR-vis range. A clean quartz slide was used as a reference and the sample was taken with the same parameters as the reference.

## FTIR Spectroscopy

To cover the mid-infrared (MIR) range, the spectra were also performed on a Br"uker Vertex 80v Fourier transform spectrometer equipped with a KBr beamsplitter and a liquid nitrogen cooled mercury-cadmium-telluride (MCT) detector. We used a resolution of 4 $cm^{-1}$, a HeNe modulation frequency of 40 kHz, and 1024 scans were averaged.

Intrinsic silicon (resistivity $> 5000\ \Omega\,\text{cm}$, 650 $\mu$m thick) was used as the substrate for the MIR range. Due to the substrates thickness, interference fringes were present in the spectra and had to be removed post-acquisition. Absorbance has been computed as $A = -\log(I/I_0)$, where $I$ is the sample single beam spectrum and $I_0$ is the reference.

### *Post-acquisition treatment*

We adapted a procedure to remove interference fringes described by Griffiths and de Haseth [5]. A forward digital Fourier transform of the absorbance data was computed, and spikes corresponding to the interference fringes were replaced by the mean value of the neighbouring points. An inverse digital Fourier transform was then performed to recover the spectrum.

Baseline was taken on a restricted window between 2000 and 635 $cm^{-1}$. A fourth order polynomial was fitted through points selected where no bands were observed, and subtracted from the original data. Lower order polynomials yielded unsatisfying agreement.

## Fitting of the Fano model

Fitting was performed with OriginLab Origin Pro 8.5 software. A custom fitting equation was defined as:

$$\sigma = \frac{A\left(q + 2\left(E - E_0\right)/\Gamma\right)^2}{1 + 2\left(E - E_0\right)/\Gamma^2}. \qquad (1)$$

The $\Gamma$, $E_0$, $q$ and $A$ parameters were allowed to vary during the fitting process.

## Raman Spectroscopy

The Raman setup was custom built with excitation laser lines at 488 nm (Kr/Ar ions laser) and 633 nm (HeNe laser). The Raman scattering signal is collected by a 50× objective mounted on a microscope and detected through a Jobin-Yvon spectrometer (model Triax 550) equipped with a nitrogen-cooled Si CCD (256×1024 pixels, Jobin-Yvon). Spot size was about 1.5 $\mu m^2$.

The laser power on the sample was adjusted to only $\sim$ 12 $\mu$W to avoid de-doping by desorption from the carbon nanotubes. We acquired a spectral domain between 1200-1700 $cm^{-1}$ in the D- and G-band regions of the SWNTs with a resolution of $\pm 1$ $cm^{-1}$.

### *Post-acquisition treatment*

Spurious rays were removed and the data interpolated linearly. A low pass FFT filter was finally applied to smooth the data.

# RESULTS

## Raman spectra

Fig. S1 shows the Raman spectra of SWNTs after purification, after annealing under high vacuum at 1100 K, after doping with DDQ, $FeCl_3$ and $SOCl_2$. At 488 nm, it is exclusively the semiconducting species that are in resonance [6]. The main features of the spectra is the so-called G-band at $\sim 1560$ and 1580 $cm^{-1}$ belonging to the tangential modes of the nanotubes, and a very faint D-band at $\sim 1335$ $cm^{-1}$ related to defects in the sidewalls. No meaningful differences between the spectra are observed. The weakness of the D-band indicates that the semiconducting nanotubes are not damaged.

The Raman spectra produced with an excitation line of 633 nm are shown in Fig. S2 for the various states

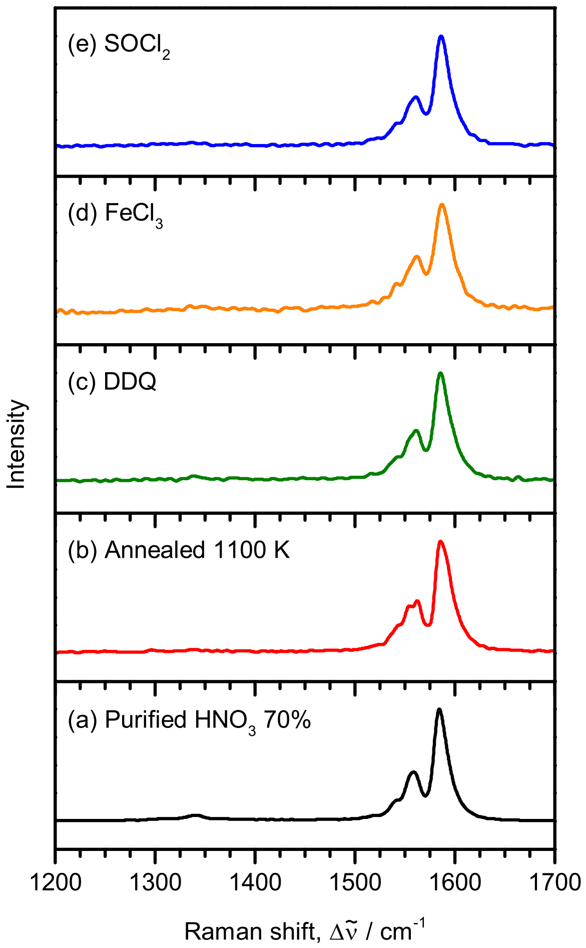


FIG. S1. Raman spectra of SWNTs films with excitation at 488 nm. (a) Purified $HNO_3$ 70%, (b) Annealed under high vacuum at 1100 K, (c) DDQ, (d) $FeCl_3$, (e) $SOCl_2$.

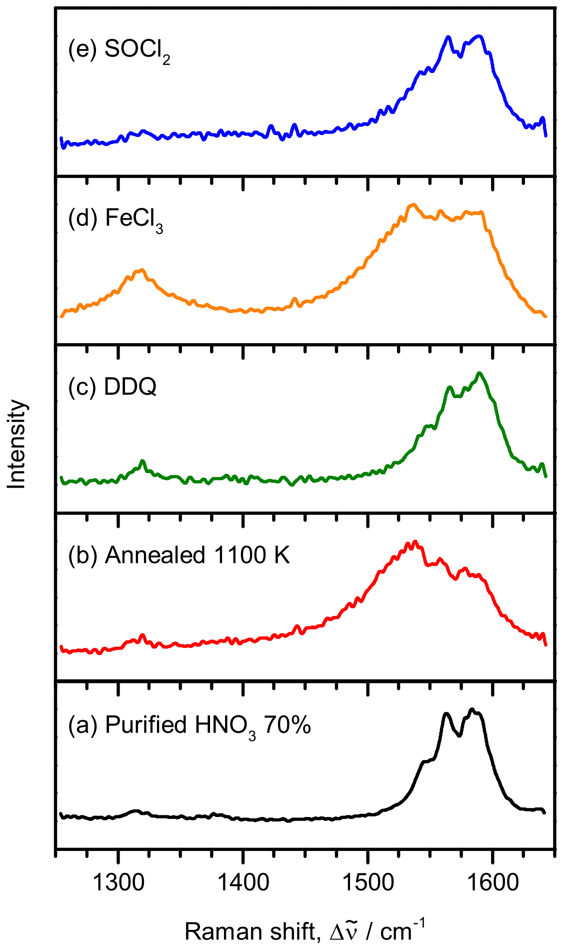


FIG. S2. Raman spectra of SWNTs films with excitation at 633 nm. (a) Purified $HNO_3$ 70%, (b) Annealed under high vacuum at 1100 K, (c) DDQ, (d) $FeCl_3$, (e) $SOCl_2$.

of SWNTs (purified, annealed, doped with DDQ, $FeCl_3$ and $SOCl_2$). At this wavelength, it is mostly the metallic species that are excited [6]. The G-band is much broader than for the semiconducting species. This broad profile is known and ascribed to a Kohn anomaly. The general shape of the G-band is dependent on the doping state of the SWNTs [7]. It becomes broader in the intrinsic state and narrower when $p$ doped. The D-band is more acute than for the semiconducting species, but varies also from a doping state to another. The spectrum in Fig. S2(a) was taken after purification with concentrated nitric acid, a strong oxidizer. It is not surprising then to note that the G-band is narrow, indicating that the nanotubes are in a doped state. Fig. S2(b) was taken in the intrinsic state after annealing, it is at this point that the G-band is the broadest. The spectra Fig. S2(c) to (d) exhibit a narrow G-band which indicates $p$ doping.

Bromophenyl functionalization of SWNTs was assessed by resonance Raman spectroscopy. An increase in the ratio of the D-band with respect to the G-band is

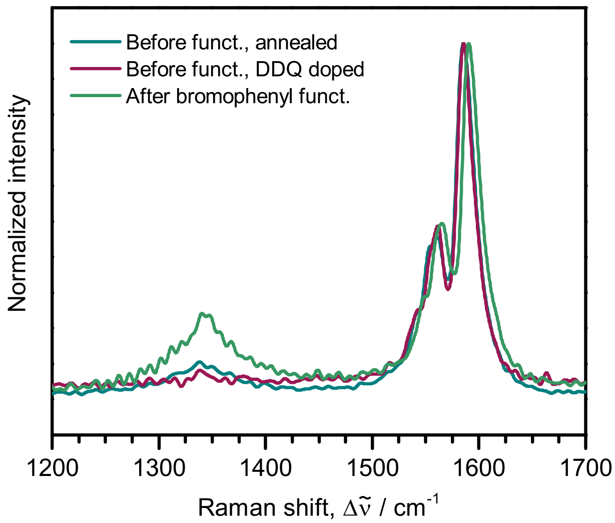


FIG. S3. Characterization by Raman spectroscopy of SWNTs films before and after bromophenyl functionalization with excitation at 488 nm.

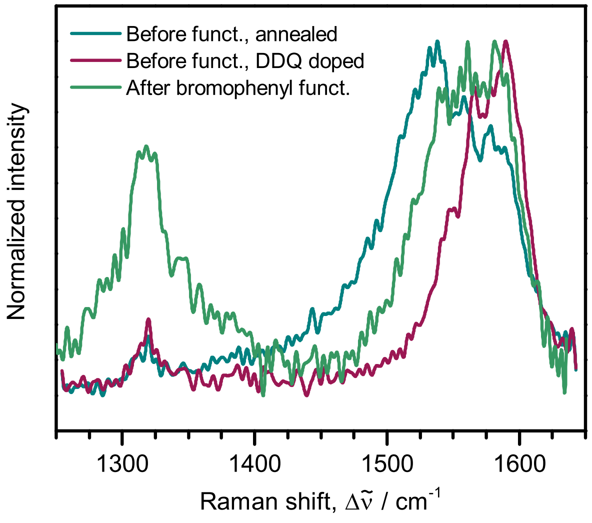


FIG. S4. Characterization by Raman spectroscopy of SWNTs films before and after bromophenyl functionalization with excitation at 633 nm.

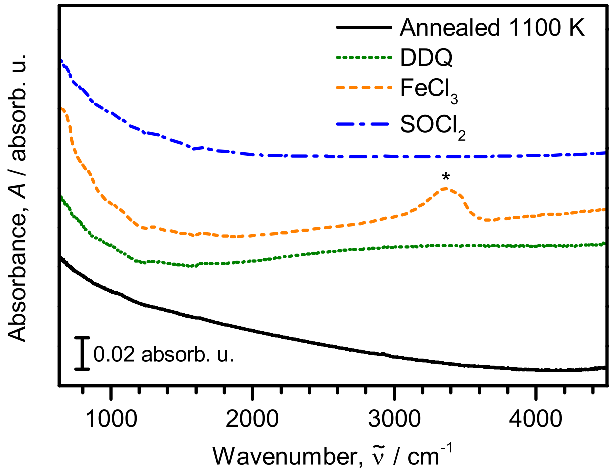


FIG. S5. Wider scale of the MIR spectra presented in Figure 2 of the main text. Starred (*) peak belong to vibrations of $FeCl_3$. Spectra are translated for clarity.

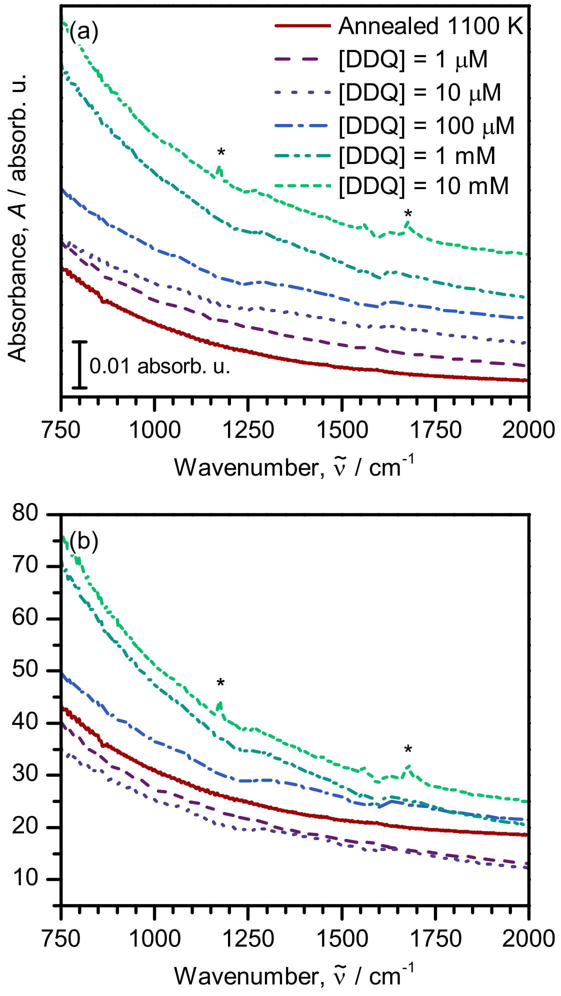


FIG. S6. MIR spectra of SWNT films as a function of [DDQ] in the acetonitrile doping solution. Starred peaks (*) belong to vibrations of DDQ. (a) Spectra translated for clarity. (b) Spectra without translation.

indicative of disorder in the SWNT sidewalls. Our spectra at 488 and 633 nm (Fig. S3 and Fig. S4) indeed show that semiconducting and metallic species are significantly damaged by the covalent grafting of bromophenyl groups, since the D-band increases in intensity compared to the normalized G-band after the functionalization step. For sakes of comparison, spectra of annealed and DDQ doped SWNTs before functionalization are also shown.

### Wider MIR spectra of the dopants

In Fig. S5, it is shown that the SWNTs annealed under high vacuum at 1100 K present a featureless spectrum (black curve). The background is rising toward the low energy end of the spectrum, which is due to the continuum of electronic states discussed in the main text. The green curve (SWNTs doped with DDQ) in Fig. S5 presents a very broad and rising feature at higher energies. The orange curve which belongs to SWNTs doped with $FeCl_3$ has also this broad feature, but also a band centered at $\sim 3300$ cm$^{-1}$. The latter band is due to the hydration of the $FeCl_3$. Finally, the blue curve (SWNTs doped with $SOCl_2$) is mostly featureless.

### MIR spectra vs. [DDQ]

We have verified the dependence of the MIR Fano resonance upon the dopant concentration in solution. We

immersed the sample in a series of solutions with concentrations ranging over four orders of magnitude (1 $\mu$M to 10 mM) starting with the less concentrated one (30 min. each). The sample was dried in a $N_2$ stream at each step. For every concentration, an MIR spectrum was taken with the same parameters as stated above. Fig. S6 shows the evolution of the spectra with the concentration of DDQ in solution. The red curve is the annealed state (high vacuum, 1100 K) and is featureless. As the concentration increases, kinks at the phonon modes energies ($\sim$1600, $\sim$1250 cm$^{-1}$ start to appear and become more acute (purple to blue to green curves). Finally, the green curve presents molecular vibrations from the DDQ molecules (1175, 1560 and 1680 cm$^{-1}$). Furthermore, the FIR band at low energy becomes steeper as the DDQ concentration is increased, indicating that more free carriers are present in the SWNTs.

* r.martel@umontreal.ca

[1] J. Liu, A. G. Rinzler, H. Dai, J. H. Hafner, R. K. Bradley, P. J. Boul, A. Lu, T. Iverson, K. Shelimov, C. B. Huffman, F. Rodriguez-Macias, Y.-S. Shon, T. R. Lee, D. Colbert, and R. E. Smalley, Science **280**, 1253 (1998).

[2] Z. Wu, Z. Chen, X. Du, J. M. Logan, J. Sippel, M. Nikolou, K. Katalin, J. R. Reynolds, D. B. Tanner, A. F. Hebard, and A. G. Rinzler, Science **305**, 1273 (2004).

[3] C. M. Aguirre, P. L. Levesque, M. Paillet, F. Lapointe, B. C. St-Antoine, P. Desjardins, and R. Martel, Adv. Mater. **21**, 3087 (2009).

[4] C. A. Dyke and J. M. Tour, Nano Lett. **3**, 1215 (2003).

[5] P. R. Griffiths and J. A. de Haseth, *Fourier Transform Infrared Spectrometry*, 2nd ed., Chemical Analysis, Vol. 171 (John Wiley & Sons, Inc., New York, 2007) p. 255.

[6] H. Kataura, Y. Kumazawa, Y. Maniwa, I. Umezu, S. Suzuki, Y. Ohtsuka, and Y. Achiba, Synth. Met. **103**, 2555 (1999).

[7] E. Anglaret, F. Dragin, A. Pnicaud, and R. Martel, J. Phys. Chem. B **110**, 3949 (2006).
